# Supplementary material for: Randomized polynomial-time equivalence between determinant and trace-IMM equivalence tests
Source: arXiv:2006.08272 source file (2020-06-15)
Supplement: Supplementary file 1 [file secappendix_comparison.tex]

\section{Algebra isomorphism and multilinear equivalence testing}\label{subsec: intro algbera isomorphism and multilinear equivalence}
\textbf{Algebra isomorphism}: An algebra over $\F$ with basis $\{E_1, \ldots, E_r\}$ is represented by its structure table $M$ which is a $r\times r\times r$ three dimensional array such that $E_i\cdot E_j = \sum_{u\in [r]} M(i,j,u)E_u$. In the algebra isomorphism problem the objective is to determine whether two algebras $\CAL{A}_1$ and $\CAL{A}_2$ over $\F$ given by its structure table are isomorphic, and if yes then also output an isomorphism from $\CAL{A}_1$ to $\CAL{A}_2$. Recently \cite{GrowchowQ19,FutornyGLS2019} showed that  over $\F$ the algebra isomorphism problem and multilinear equivalence testing are equivalent. \\
\\
\textbf{Algebra isomorphism to multilinear equivalence}: In particular,  \cite{FutornyGLS2019} reduces the problem of testing whether two algebras $\CAL{A}_1$ and $\CAL{A}_2$ of dimension $r$ over $\F$ are isomorphic to testing whether two degree $3$, $n$ variate set-multilinear polynomials $f_{\CAL{A}_1}$ and $f_{\CAL{A}_2}$ are multilinearly equivalent, where $n = r^{O(1)}$. In Theorem \ref{theorem: reduction from fmai to emi} we reduce an important special instance of the algebra isomorphism problem, namely $\FMAI$, in randomized polynomial time to an important special instance of degree three multilinear equivalence testing, namely degree 3 $\MEIMM$. The reduction in \cite{FutornyGLS2019} when applied as it is to  $\FMAI$, that is $\CAL{A}_1 = \CAL{A}$ as in Theorem \ref{theorem: reduction from fmai to emi} and $\CAL{A}_2 = \CAL{M}_w$ with the canonical basis of $\CAL{M}_w$\footnote{The canonical basis of $\CAL{M}_w$ is $\{E_{i,j}\mid E_{i,j} \in \CAL{M}_w,$ and the $(i,j)$-th entry of $E_{i,j}$ is one and the remaining entries of $E_{i,j}$ are zero, for $i,j\in [w]\}$.}, reduces $\FMAI$ to testing whether two degree $3$, $w^{O(1)}$ variate set-multilinear polynomials $f_{\CAL{A}}$ and $f_{\CAL{M}_w}$ are multilinearly equivalent. But the polynomial $f_{\CAL{M}_w}$ is not equal to $\IMM_{w',3}$ for any $w'\in \N$.\\
\\
\textbf{Multilinear equivalence to algebra isomorphism}: In the reverse direction \cite{GrowchowQ19} reduced the problem of testing whether two homogeneous degree $d$ set-multilinear polynomials in $\vecx_0, \ldots, \vecx_{d-1}$ variables are multilinearly equivalent to testing whether two algebras of dimension $O(d^2w^{d-1})$ are isomorphic. In contrast, we use Theorem \ref{theorem: reduction from equivalence testing of trace to det} (see remark thereafter) and the reduction in \cite{GargGKS19} (from $\EDET$ to $\FMAI$) to show that multilinear equivalence testing of $\IMM_{w,d}$ reduces in randomized polynomial time to testing whether a matrix algebra of dimension $w^2$ is isomorphic to $\CAL{M}_w$. The results in \cite{FutornyGLS2019,GrowchowQ19} show that algebra isomorphism and degree three multilinear equivalence testing are polynomial time equivalent, but our results show that their special instances $\FMAI$ and degree $3$ $\MEIMM$ are randomized polynomial time equivalent. \\
\\
\textbf{A naive reduction}: A natural way to associate a degree $3$ set-multilinear polynomial $f_{\CAL{A}}$ with an algebra $\CAL{A}$ specified by its basis $\{E_1, \ldots, E_r\}$ and its structure table $M$ is as follows: $f_{\CAL{A}}$ is a set-multilinear polynomial in $\vecy_0, \vecy_1, \vecy_2$ variables, where $\vecy_k = \{y_{k,1}, \ldots, y_{k,r}\}$ for $k\in [0,2]$ and the coefficient of $y_{1,i}y_{2,j}y_{3,u}$ is equal to $M(i,j,u)$ for $i,j,u\in [r]$. Thus, a naive reduction from algebra isomorphism to degree three multilinear equivalence testing would be to test whether the polynomials $f_{\CAL{A}_1}$ and $f_{\CAL{A}_2}$ constructed from the input algebras $\CAL{A}_1$ and $\CAL{A}_2$ (as explained above) are multilinearly equivalent. But it is not clear whether $\CAL{A}_1$ and $\CAL{A}_2$ being isomorphic implies $f_{\CAL{A}_1}$ and $f_{\CAL{A}_2}$ are multilinearly equivalent or the vice-versa. Similarly, for $\FMAI$ an easy observation shows that $f_{\CAL{M}_w}$ constructed (as above) from $\CAL{M}_w$ with its canonical basis is equal to $\textnormal{Trace}(Q_0\cdot Q_1\cdot Q_2^T)$\footnote{Here $\vecy_k = \vecx_k$ for $k\in [0,2]$.}. Hence, in the above naive reduction replacing  $\CAL{A}_2$ with $\CAL{M}_w$ specified by its canonical basis might reduce $\FMAI$ to degree $3$ $\MEIMM$ but the correctness of this reduction is not known. The reductions in \cite{FutornyGLS2019} and in our work (Theorem \ref{theorem: reduction from fmai to emi}) are different from this. While the reduction in \cite{FutornyGLS2019} is inspired from the above reduction and constructs the polynomials from the structure table of the two input algebras, Theorem \ref{theorem: reduction from fmai to emi} as stated previously uses Lemma \ref{lemma: characterization of trace by its lie algebra} and a nice representation of the basis elements of $\GIMM$. A naive reduction from degree three multilinear equivalence testing to algebra isomorphism can also be thought about by associating the coefficients of the input polynomials with the entries of the structure table of two algebras. But in this case, a structure table obtained from a degree three set-multilinear polynomial does not always correspond to a valid algebra \footnote{The associativity of the multiplication does not always hold.}.\\
\\
%Moreover, even though $\CAL{A}_1$ and $\CAL{A}_2$ being isomorphic implies $f_{\CAL{A}_1}$ and $f_{\CAL{A}_2}$ are multilinearly equivalent, for the search version it is not clear how to construct an isomorphism from $\CAL{A}_1$ to $\CAL{A}_2$ using $B_0, B_1, B_2 \in \mathsf{GL}(r,\F)$ such that $f_{\CAL{A}_2}(\vecy_0, \vecy_1, \vecy_2) = f_{\CAL{A}_1}(B_0\vecy_0, B_1\vecy_1, B_{2}\vecy_{2})$\footnote{The matrices $B_0, B_1, B_2$ are not unique and depend on the symmetries of $f_{\CAL{A}_1}$.}.
\textbf{Degree $d$ to degree $3$ multilinear equivalence}:  The reductions in \cite{FutornyGLS2019,GrowchowQ19} also show that the problem of testing whether two homogeneous degree $d$ set-multilinear polynomials are multilinearly equivalent reduces to testing whether two homogeneous degree $3$ set-multilinear polynomials $f'$ and $g'$ in $\vecy_0,\vecy_1, \vecy_2$ variables are multilinearly equivalent in $(dw)^{O(d)}$ time, where $\vecy_k = (dw)^{O(d)}$ for $k\in [0,2]$. Theorem \ref{theorem: reduction from equivalence testing for degree d to degree 3} shows that the special instance of degree $d$ $\MEIMM$ reduces in \emph{randomized polynomial} time to degree $3$ $\MEIMM$. The result in \cite{GrowchowQ19} when applied as it is to the special case where $g = \IMM_{w,d}$ reduces $\MEIMM$ to testing whether two degree $3$ set-multilinear polynomials $f'(\vecy_0, \vecy_1, \vecy_2)$ and $g'(\vecy_0, \vecy_1,\vecy_2)$ are multilinearly equivalent where $\vecy_k = (dw^{d})^{O(1)}$. The number of $\vecy$ variables depend exponentially on $d$, and $g'(\vecy)$ which is reduced from $\IMM_{w,d}$ is not equal to $\IMM_{w',3}$ for a $w' \in \N$.\\ 
\\
\textbf{Decision version and connection with $\EDET$}: The reductions in \cite{FutornyGLS2019,GrowchowQ19} also hold for the decision versions of the two problems. In comparison, it is not clear whether the reductions in Theorems \ref{theorem: reduction from equivalence testing of trace to det} and \ref{theorem: reduction from equivalence testing for degree d to degree 3}, and the reduction from $\EDET$ to $\FMAI$ in \cite{GargGKS19} hold for their respective decision versions. As stated previously though, the first part of the reduction in Theorem \ref{theorem: reduction from fmai to emi} reduces the decision version of $\FMAI$ in deterministic polynomial time to the decision version of degree $4$ $\MEIMM$. Also Corollary \ref{corollary: equivalence of det, trace and fmai} proves that $\FMAI$ and degree $3$ $\MEIMM$ are randomized polynomials time equivalent to $\EDET$, whereas the reductions in \cite{FutornyGLS2019,GrowchowQ19} seems to have no connection with $\EDET$.
