# Supplementary material for: Randomized polynomial-time equivalence between determinant and trace-IMM equivalence tests
Source: arXiv:2006.08272 source file (2020-06-15)
Supplement: Supplementary file 2 [file secappendix_proof_of_lie_algebra.tex]

\section{Proof of Lemma \ref{theorem: lie algebra of of trace}}\label{secappendix: proof of lie algebra}
Recall the rows (corresponding to derivatives) and columns (corresponding to shifts) of matrices in $\GIMM$ are indexed by $\vecx$ variables ordered as in Section \ref{subsec: Variable ordering, notations and definitions}. As part of Claim \ref{claim: the block-diagonal spaces are in the lie algebra}, we show that $\CAL{B}_k \subseteq \GIMM$, for all $k \in [0,d-1]$. Then in Claim \ref{claim: lie algebra is constined in the block-diagonal spaces} we show that $\GIMM \subseteq \sum_{k\in [0,d-1]} \CAL{B}_k$. 
\begin{claim}\label{claim: the block-diagonal spaces are in the lie algebra}
For every $k \in [0,d-1]$, $\CAL{B}_k \subseteq \G_{\IMM}$.
\end{claim}
\begin{proof}
Let $k \in [0,d-2]$, $k$ even, and $B \in \CAL{B}_k$. Hence there is an $M \in \CAL{M}_w$ such that the $2w^2 \times 2w^2$ sub-matrix of $B$ whose rows and columns are indexed by $\vecx_{k} \uplus \vecx_{k+1}$ variables is as follows
$$ \begin{bmatrix}
     I_w \otimes M^T & \mathbf{0} \\
     \mathbf{0}  & -M \otimes I_w
    \end{bmatrix}~~.
$$
Let $M = (m_{i,j})_{i,j \in [w]}$, and $\ell_{i,j}^{(k)} = \sum_{v\in [w]} m_{v,j} x_{i,v}$ and $\ell_{i,j}^{(k+1)} = \sum_{v\in [w]} - m_{i,v} x_{v,j}$ for all $i,j \in [w]$. Further, let $Q'_k = (\ell_{i,j}^{(k)})_{i,j \in [k]}$, and $Q'_{k+1} = (\ell_{i,j}^{(k+1}))_{i,j\in [w]}$. Then Observations \ref{observation: containment of B} follows from the definition of the Lie algebra of a polynomial (Definition \ref{def:lie_algebra}) and Observation \ref{observation: structure of Q'k} follows from the structure of $Q'_k$ and $Q'_{k+1}$.
\begin{observation}\label{observation: containment of B}
The matrix $B \in \GIMM$ if and only if the following holds:
\begin{align*}\label{equation: lie algebra equation for block spaces in Lie algebra lemma }
    \sum_{i,j\in [w]} \ell_{i,j}^{(k)} \frac{\partial f}{x_{i,j}^{(k)}} ~~~+ \sum_{i,j\in [w]} \ell_{i,j}^{(k+1)} \frac{\partial f}{x_{i,j}^{(k+1)}} ~~~ &= ~~~  \textnormal{Trace}(Q_1\cdots Q_{k-1}( Q'_k\cdot Q_{k+1} +  Q_k\cdot Q'_{k+1})Q_{k+2} \cdots Q_{d-1} \\
    & = ~~~~0~.
\end{align*}
\end{observation}
\begin{observation}\label{observation: structure of Q'k}
The matrices $Q'_k$ and $Q'_{k+1}$ are such that $Q'_k = Q_k\cdot M$ and $Q'_{k+1} = -M\cdot Q_{k+1}$.
\end{observation}
From Observation \ref{observation: structure of Q'k} it follows that $Q'_k\cdot Q_{k+1} = -Q_{k}\cdot Q'_{k+1}$, and hence from Observation \ref{observation: containment of B} it follows that $B \in \G_{\IMM}$. The proofs for the remaining two cases: a) $k \in [0,d-1]$, $d$ even and $k$ odd, and b) $k = d-1$ and $d$ odd are similar.
\end{proof}
\begin{claim}\label{claim: lie algebra is constined in the block-diagonal spaces}
Let $E = (e_{ij})_{n \times n} \in \GIMM$. Then $E \in \sum_{k\in [0,d-1]}\CAL{B}_k$.
\end{claim}
Observation \ref{claim: gtrimm is block diagonal} shows that every matrix in $\GIMM$ is a block-diagonal matrix.
\begin{observation}{\label{claim: gtrimm is block diagonal}}
If $E \in \G_{\IMM}$ then $E$ is block-diagonal.
\end{observation}
\begin{proof}
Since $E \in \G_\IMM$, it satisfies the following equation. 
\begin{equation}{\label{equation:Lie Algebra equation for Tr-IMM}}
    \sum_{i,j \in [n]}e_{ij}\cdot x_{j}\cdot\frac{\partial \IMM}{\partial x_i} = 0\ \ .
\end{equation}
Equation \ref{equation:Lie Algebra equation for Tr-IMM}  can be rewritten as follows
\begin{equation}{\label{equation:main eqn split}}
\underbrace{\sum_{\substack{x_i,x_j \in \vecx_k \\ k\in[0,d-1]} }e_{ij} \cdot x_j \cdot \frac{\partial \IMM}{\partial x_i}}_{(a)}~~ + ~~~\underbrace{\sum_{\substack{x_i \in \vecx_l\ x_j \in \vecx_k \\ l,k\in [0,d-1], l \neq k}} e_{ij} \cdot x_j \cdot \frac{\partial  \IMM}{\partial x_i}}_{(b)}  = 0 .
\end{equation} 
In Equation \ref{equation:main eqn split}, term (a) corresponds to the \textit{block-diagonal entries} of $E$ and term (b) corresponds to the \textit{non block-diagonal entries} of $E$. Observe that both the terms are monomial disjoint: monomials in term (a) have variables from each variable set $\vecx_{0}, \ldots, \vecx_{d-1}$, whereas monomials in term (b) have two variables from $\vecx_{k}$ and no variable from $\vecx_{l}$ $l,k\in [0,d-1]$ and $l\neq k$. This implies terms (a) and (b) are individually equal to zero. 
\begin{align}{\label{equation: split term a are zero}}
\sum_{\substack{x_i,x_j \in \vecx_k \\ k\in[0,d-1]} }e_{ij} \cdot x_j \cdot \frac{\partial \IMM}{\partial x_i} &= 0 \\   
\sum_{\substack{x_i \in \vecx_l\ x_j \in \vecx_k \\ l,k\in [0,d-1], l \neq k}} e_{ij} \cdot x_j \cdot \frac{\partial  \IMM}{\partial x_i} &= 0.
\end{align}
Additionally the terms $x_j \frac{\partial \IMM}{\partial x_i}$ and $x_{j'} \frac{\partial \IMM}{\partial x_{i'}}$ in (b) are monomial disjoint whenever $(l,k) \neq (l',k')$ where $x_i \in \vecx_l, x_j \in \vecx_k$ and $x_i' \in \vecx_{l'}, x_j' \in \vecx_{k'}$. Thus for every pair $(l,k)$ with $l \neq k$ we have 
\begin{align}{\label{equation: split terms for non-block diagonal}}
\sum_{\substack{l \neq k, l,k\in [0,d-1]\\x_i \in \vecx_l\ x_j \in \vecx_k;}} e_{ij} \cdot x_j \cdot \frac{\partial  \IMM}{\partial x_i} &= 0.
\end{align}
In Equation \ref{equation: split terms for non-block diagonal}, group the coefficients of the term $\frac{\partial \IMM}{\partial x_i}$ together and rewrite it as
\begin{equation}{\label{equation: non block diagonal space linear form}}
     \sum_{x_i \in \vecx_l} L_{x_i}^{(l,k)}\frac{\partial \IMM}{\partial x_i} = 0
\end{equation}
where $L_{x_i}^{(l,k)}(\vecx_k)$ is a linear form in the $\vecx_k$ variables. The proof concludes by showing that $L_{x_i}^{(l,k)}$ is identically zero. \vspace{0.1in}

Let $x_i = x_{p,q}^{(l)}$, that is it is the $(p,q)$-th entry of $Q_l$, where $p,q \in [w]$. Also let $Q'_{l}$ be a $w \times w$ matrix whose $(p,q)$-th entry is the linear form $L_{x_i}^{(l,k)}$. Then from Equation \ref{equation: non block diagonal space linear form}.
\begin{equation}\label{equation: non block diagonal space linear form with trace}
    \sum_{x_i \in \vecx_l}L_{x_i}\frac{\partial \IMM}{\partial x_i}~ =~ \textnormal{Trace}(Q_0 \ldots Q'_{l} \ldots Q_{d-1}) ~=~ 0~.
\end{equation} 
Now suppose for contradiction $L_{x_i}^{(l,k)}\neq 0$. Then there is an $x_j \in \vecx_k$ such that the coefficient of $x_j$ in $L_{x_i}^{(l,k)}$ is not equal to zero. Choose a monomial $\mu$ in $\IMM_{w,d}$ such that $\mu$ contains the variable $x_i$; $\mu$ could contain $x_j$ but not necessary. In Equation \ref{equation: non block diagonal space linear form with trace} set all the variables to zero except the variable $x_j$ and the variables appearing in $\mu$. Under this assignment the polynomial computed by $\textnormal{Trace}(Q_0 \ldots Q'_l \ldots Q_{d-1})$ is non-zero as the linear form $L_{x_i}^{(p,q)}(\mathbf{x}_q) \neq 0$. But $\textnormal{Trace}(Q_0 \ldots Q'_l \ldots Q_{d-1})$ is a zero polynomial which is a contradiction.
\end{proof}
Thus from Observation \ref{claim: gtrimm is block diagonal} we conclude that the entries of $E\in \GIMM$ satisfy
\begin{equation}\label{equation: for block-diagonal}
    \sum_{\substack{x_i,x_j \in \vecx_k \\ k\in[0,d-1]} }e_{ij} \cdot x_j \cdot \frac{\partial \IMM}{\partial x_i} = 0
\end{equation}
Rewrite Equation \ref{equation: for block-diagonal} as follows
\begin{equation}{\label{equation: split block diagonal}}
   \underbrace{\sum_{i \in [n]} e_{ii} \cdot x_i \cdot\frac{\partial  \IMM}{\partial x_i}}_{(a)}~~ +~~  \underbrace{\sum_{\substack{x_i \neq x_j \\ x_i,x_j \in \vecx_k} }e_{ij} \cdot x_j \cdot \frac{\partial \IMM}{\partial x_i}}_{(b)}  = 0.
\end{equation}
Again in Equation \ref{equation: split block diagonal} the monomials in terms (a) and (b) are disjoint: monomials in term (a) are path monomials and those in (b) are non-path monomials.
Hence, 
\begin{equation}
  \sum_{i \in [n]} e_{ii} \cdot x_i \cdot\frac{\partial  \IMM}{\partial x_i} = 0~~~~\textnormal{and}  
\end{equation}
\begin{equation}
\sum_{\substack{x_i \neq x_j \\ x_i,x_j \in \vecx_k} }e_{ij} \cdot x_j \cdot \frac{\partial \IMM}{\partial x_i} = 0 .
\end{equation}
Let $E_d$ be an $n\times n$ diagonal matrix such that its diagonal entries are equal to the diagonal entries of $E$, and $E_b$ be a block-diagonal matrix whose diagonal entries are zero, and its remaining entries are equal to $E$. In particular, $E = E_d +E_b$. In Observations \ref{} and \ref{} we argue $E_d$ and $E_b$ belong to $\sum_{k\in [0,d-1]}\CAL{B}_k$ respectively.
\begin{observation}
The matrix $E_d \in \sum_{k\in [0,d-1]}\CAL{B}_k$
\end{observation}
\begin{proof}
\emph{a) $d$ even}: Corresponding to every path monomial $\mu = x_{i_0,i_1}^{(0)}\cdot x_{i_1,i_2}^{(1)}\ldots x_{i_{d-1},i_0}^{(d-1)}$, the entries of $E_d$ satisfy $\sum_{k=0}^{d-1} e_{i_{k},i_{k+1}}^{(k)} = 0$.  Here the entry  $e_{i_{k},i_{k+1}}^{(k)}$ is the diagonal entry of $E_d$ indexed by the variable $x_{i_k,i_{k+1}}^{(k+1)}$. In particular for $i_0 = i_1 = \ldots = i_{d-1} = i$, where $i\in [w]$ we have
\begin{equation}\label{equation: for direct path monomial}
    \sum_{k=0}^{d-1}e_{i,i}^{(k)} = 0 ~, 
\end{equation}
and for some $\ell \in [0,d-1]$ and $i,j\in [w]$,
\begin{equation}\label{equation: for indirect path monomial}
    \sum_{k=0}^{\ell-1}e_{i,i}^{(k)} + e_{i,j}^{(\ell)} + e_{j,i}^{(\ell+1)} + \sum_{k=\ell+2}^{d-1}e_{i,i}^{(k)}  = 0 ~. 
\end{equation}
From Equations \ref{equation: for direct path monomial} and \ref{equation: for indirect path monomial} we infer that for $\ell\in [0,d-1]$, $i,j\in [w]$,
\begin{equation}\label{equation: for indirect path monomial}
   e_{i,i}^{(\ell)} + e_{i,i}^{(\ell+1)}   =  e_{i,j}^{(\ell)} + e_{j,i}^{(\ell+1)} ~.
\end{equation}

\end{proof}

New part ......\\
\\

The following corollary follows easily from the disjointness of the terms (a) and (b) of Equation~\ref{equation:main eqn split} and Claim~\ref{claim: gtrimm is block diagonal}. 

\begin{corollary}{\label{corollary: wb and wd}}
Let $\CAL{W}_b$ denoted the space spanned by the matrices in $\G_{\IMM}$ whose diagonal entries are 0 and $\CAL{W}_d$ denote the space spanned by the diagonal matrices in $\G_{\IMM}$. Then $\G_{\IMM} = \CAL{W}_b \oplus \CAL{W}_d$. 
\end{corollary} 
\par We now analyze the structure of the space $\CAL{W}_b$. Consider $B = (b_{ij})_{n \times n} \in \CAL{W}_b$. Clearly, it satisfies the following equation.
\begin{equation}{\label{eq:bd_eqn}}
    \sum_{i,j \in [n]}b_{ij}x_j \frac{\partial \IMM}{\partial x_j} = 0\ \ .
\end{equation}
Since $B \in \CAL{W}_b$, the only terms in the above equation with non-zero coefficients are those for which $x_i,x_j \in \vecx_k$ for some $k \in [0,d-1]$.  We now make the following observation which can be easily verified. 

\begin{observation}{\label{obs:bd1}}
Consider $x_i = x_{pq}^{(k)}$ and $x_j = x_{rs}^{(k)}$ where $k \in [0,d-1]$ and $p,q,r,s \in [w]$. Further, let $p \neq r$ and $q \neq s$. The term $x_j\cdot\frac{\partial \IMM}{\partial x_i}$  does not share a monomial with any other term in Equation~\ref{eq:bd_eqn}, implying the coefficients of any monomial in these terms are 0.
\end{observation}

We now consider at the remaining terms for which either $p = r$ or $q = s$. For this purpose, it is useful to define the notion of monomials broken at $k$-th interface. 
\\~
\par{\textbf{Monomials broken at $k$-th interface:}}
A monomial broken at the $k$-th interface is of the form $x_{i_0i_1}\cdot x_{i_1i_2}\ldots x_{i_{k-1}i_{k}}\cdot x_{i_{k}^{'}i_{k+1}}\ \ldots  x_{i_{d-1}i_0}\ \forall k \in [0,d-1]$ where $i_{k+1} \neq i_{k+1}^{'}$. 

Any monomial in the term $x_{ps}^{(k)}\cdot\frac{\partial \IMM}{\partial x_{pq}^{(k)}}$ or $x_{qt}^{(k+1)}\cdot\frac{\partial \IMM}{\partial x_{st}^{(k+1)}}$ is a monomial broken at $k$-th interface. In fact it can be verified that any monomial broken at the $k$-th interface is contained in one of the terms $x_{ps}^{(k)}\cdot\frac{\partial \IMM}{\partial x_{pq}^{(k)}}$ or $x_{qt}^{(k+1)}\cdot\frac{\partial \IMM}{\partial x_{st}^{(k+1)}}$ where $p,q,s,t \in [w]$. Hence we make the following observation. 

\begin{observation}{\label{obs:disjointness of monomials broken at kth interface}}
Let $M_k$ denote the set of all monomials broken at $k$-th interface, where $k \in [d]$. Then $i \neq j$ implies, $M_i$ and $M_j$ are disjoint.
\end{observation}
